# Supplementary material for: Latent Su-Schrieffer-Heeger models
Source: arXiv:2310.07619 source file (2023-10-11)

(a)

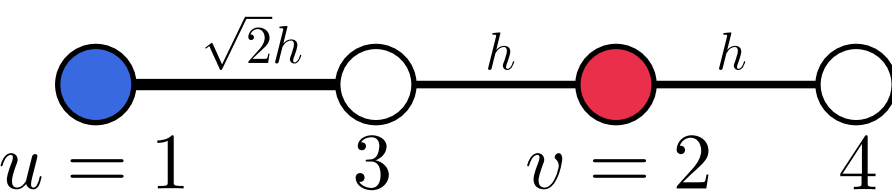

(b)

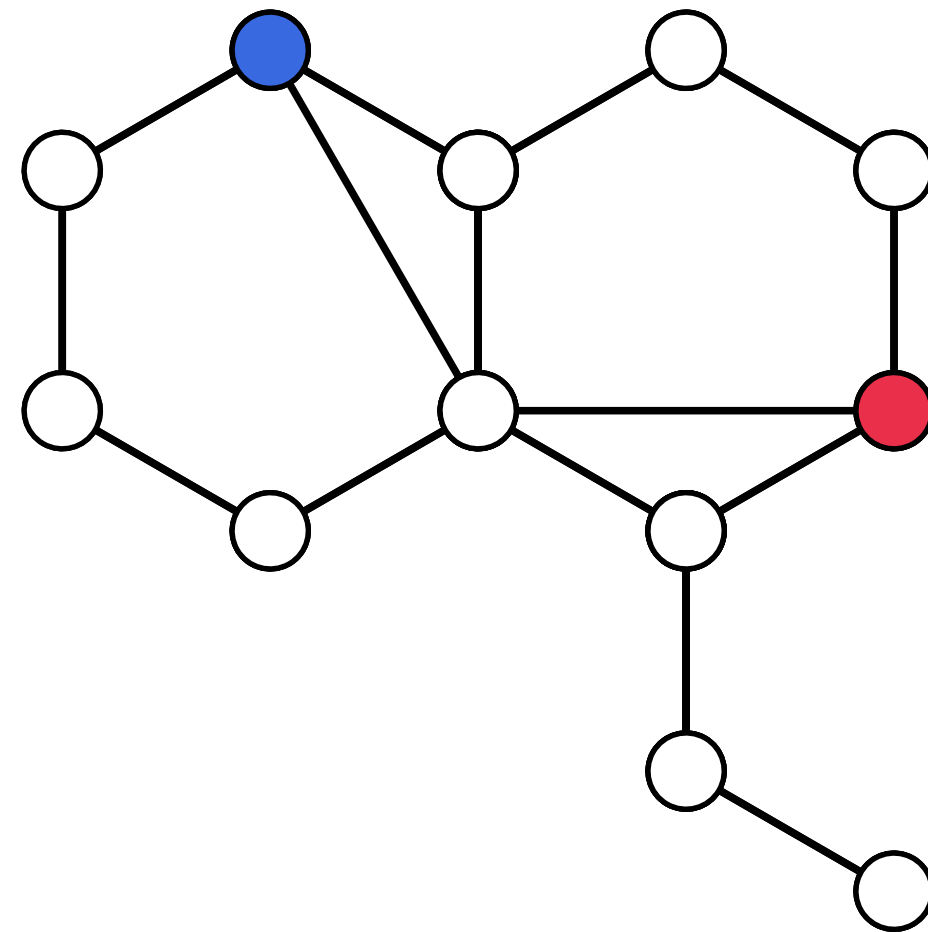

(c)

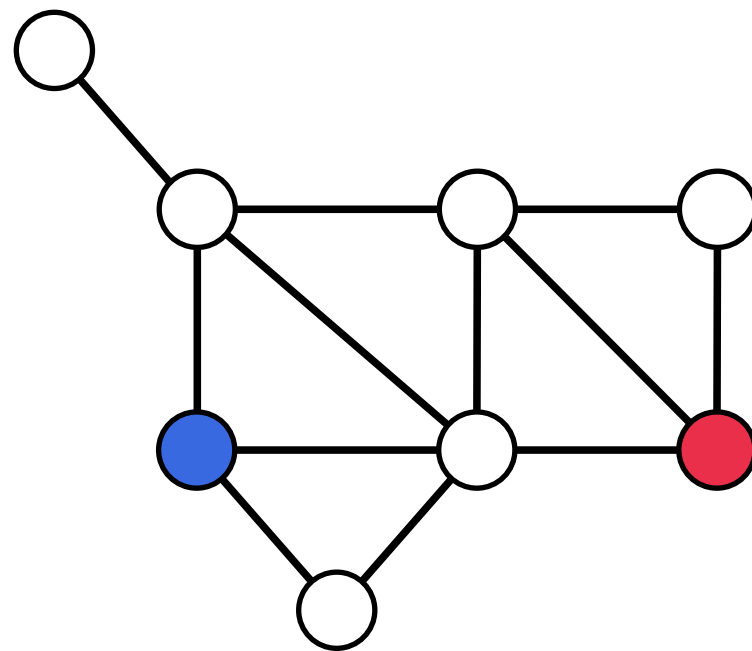

(d)

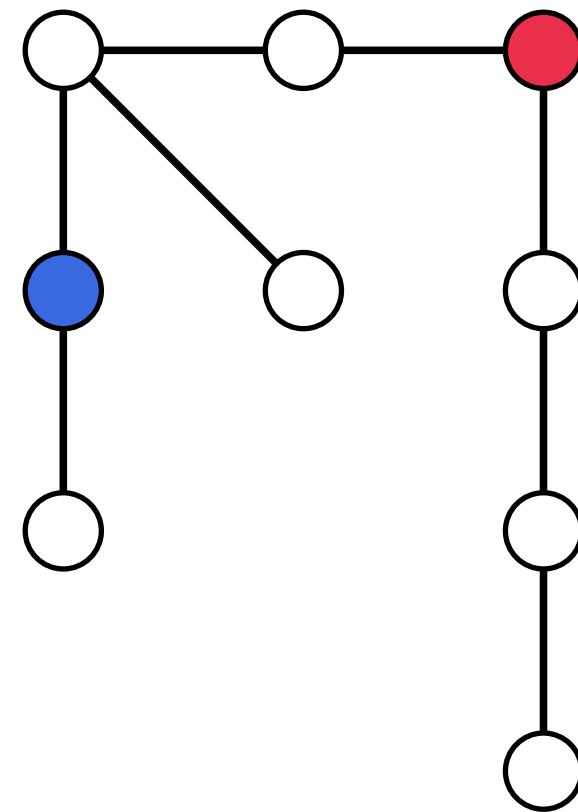

(e)

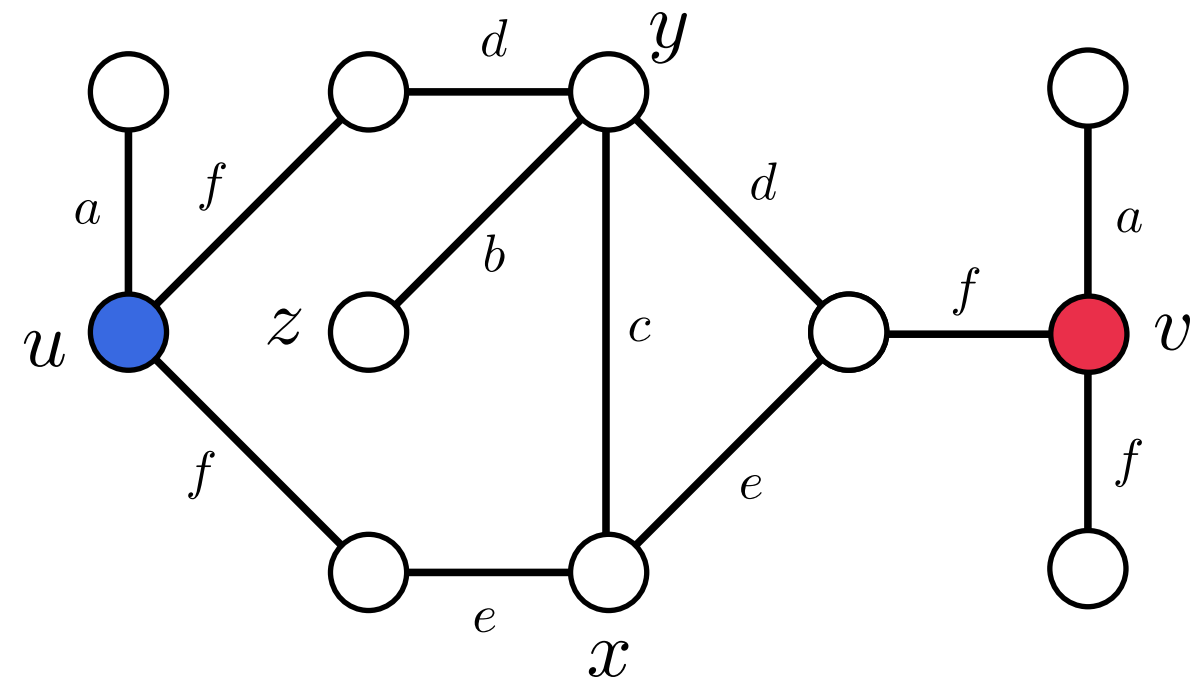

Supplement: Supplementary file 1 [file SuppMatLatSymm.pdf]
